# Supplementary material for: Detecting LLM Fact-conflicting Hallucinations Enhanced by Temporal-logic-based Reasoning
Source: arXiv:2502.13416 source file (2025-02-19)
Supplement: Supplementary file 1 [file 9.appendix.tex]

\subsection{Correctness of the encoding rules}
\label{app:correctness}

\ThemSoundAndComplete*
\begin{proof} By a case analysis of the encoding rules and semantic definitions: 

\begin{enumerate}[itemsep=1.5em,leftmargin=!]
\vspace{1em}
\item Atomic Proposition: 
{
\small 
\begin{align*}
\frac{
\begin{matrix}
\widetilde{\drule} = [\nmNEW(\interval) \hornarrow \nm\_{\m{TS}}(\interval).]
\end{matrix}
}{\encoding {\nm}{\nmNEW}{\widetilde{\drule}}}\ [\trans\text{-}\m{AP}]
\end{align*}
\vspace{-1mm}
\begin{align*}
\input{sementics_rules/AP}
\end{align*}
\vspace{-8mm}
}

In   
$[\trans\text{-}\m{AP}]$, with $\nm$, 
$\forall \interval.~\llbracket \nmNEW(I) \rrbracket_{\Prolog} {=} \m{true}$, 
its premise indicates that 
$\llbracket  \nm_{\m{TS}}(\interval)\rrbracket_{\history} {=} \m{true}$. 
Next, from the semantic definition, we have 
$\forall  \timepoint\,{\in}\,\interval, (\history, \timepoint) {\models} \nm$; thus, the rule is sound. 
\\
From the semantic definition, $\forall   (\history, \timepoint) {\models} \nm$, it indicates that $\exists\interval.~\llbracket  \nm_{\m{TS}}(\interval)\rrbracket_{\history} {=} \m{true} ~\m{and}~
\timepoint\,{\in}\,\interval$.  
Next, from $[\trans\text{-}\m{AP}]$, we obtain 
$\llbracket \nmNEW(I) \rrbracket_{\Prolog} {=} \m{true}$; thus, the rule is complete.

\item  Finally:
{
\small 
\begin{align*}
\frac{
\begin{matrix}
\widetilde{\drule} {=} 
[\nmNEW([\interval^\prime_\m{start}\text{-}\interval_{\m{end}}, \interval^\prime_\m{end}\text{-}\interval_{\m{start}}]) \hornarrow \nm(\interval^\prime).]
\end{matrix}
}{\encoding {\mathcal{F}_\interval\,\mtl}{\nmNEW}{\widetilde{\drule} }}\ [\trans\text{-}\m{Finally}]
\end{align*}
\vspace{-1mm}
\begin{align*}
\input{sementics_rules/Finally_sementics}
\end{align*}
\vspace{-8mm}
}

In $[\trans\text{-}\m{Finally}]$  with 
$\mathcal{F}_{[\Istart, \Iend]}\,\mtl$, \\
$\forall \interval^{\prime\prime}.~\llbracket \nmNEW(\interval^{\prime\prime}) \rrbracket_{\Prolog} {=} \m{true}$, 
its premise indicates that \\
$\llbracket  \nm([\interval^{\prime\prime}_\m{start}\plus\Iend, \interval^{\prime\prime}_\m{end}\plus\Istart])\rrbracket_{\history} {=} \m{true}$, 
which means that $\forall \timepoint \,{\in}\,\interval^{\prime\prime}$, there exists $\distance\,{\in}\,[\Istart, \Iend]$ such that $(\history, \timepoint\plus\distance) {\models} \mtl$
\\
Next, from the semantic definition, we have \\
$\forall  \timepoint\,{\in}\,\interval^{\prime\prime}, 
(\history, \timepoint) {\models} \mathcal{F}_{[\Istart, \Iend]}\,\mtl$; thus the rule is sound. \\
From the semantic definition, $\forall   
(\history, \timepoint) {\models} \mathcal{F}_{[\Istart, \Iend]}\,\mtl$; it indicates that 
$\exists \distance\,{\in}\,[\Istart, \Iend] ~\m{and}~ (\history, \timepoint\plus\distance)\models\mtl$, 
which means that 
$\exists \interval^\prime.~ \timepoint\plus\distance\,{\in}\, \interval^\prime ~\m{and} ~\llbracket \nm(\interval^\prime) \rrbracket_{\Prolog} {=} \m{true}$
\\
Next, from $[\trans\text{-}\m{Finally}]$, 
we obtain \\
$\llbracket \nmNEW([\interval^\prime_\m{start}\text{-}\Iend, \interval^\prime_\m{end}\text{-}\Istart]) \rrbracket_{\Prolog} {=} \m{true}$,  and thus \\
$\timepoint\,{\in}\,[\interval^\prime_\m{start}\text{-}\Iend, \interval^\prime_\m{end}\text{-}\Istart]$; 
thus, the rule is complete. 

\item  Globally:
{
\small 
\begin{align*}
\frac{
\begin{matrix}
\widetilde{\drule} {=} 
[\nmNEW([\interval^\prime_\m{start}\text{-}\interval_{\m{start}}, \interval^\prime_\m{end}\text{-}\interval_{\m{end}}]) \hornarrow \nm(\interval^\prime).]
\end{matrix}
}{\encoding {\mathcal{G}_\interval\,\mtl}{\nmNEW}{\widetilde{\drule} }}\ [\trans\text{-}\m{Globally}]
\end{align*}
\vspace{-1mm}
\begin{align*}
\input{sementics_rules/Globally_sementic}
\end{align*}
\vspace{-8mm}
}

In $[\trans\text{-}\m{Globally}]$  with 
$\mathcal{G}_{[\Istart, \Iend]}\,\mtl$, \\
$\forall \interval^{\prime\prime}.~\llbracket \nmNEW(\interval^{\prime\prime}) \rrbracket_{\Prolog} {=} \m{true}$, 
its premise indicates that \\
$\llbracket  \nm([\interval^{\prime\prime}_\m{start}\plus\Istart, \interval^{\prime\prime}_\m{end}\plus\Iend])\rrbracket_{\history} {=} \m{true}$, which means that $\forall \timepoint \,{\in}\,\interval^{\prime\prime}$, for all $\distance\,{\in}\,[\Istart, \Iend]$ such that $(\history, \timepoint\plus\distance) {\models} \mtl$. \\
Next, from the semantic definition, we have \\
$\forall  \timepoint\,{\in}\,\interval^{\prime\prime}, 
(\history, \timepoint) {\models} \mathcal{G}_{[\Istart, \Iend]}\,\mtl$; thus the rule is sound. \\
From the semantic definition, $\forall   
(\history, \timepoint) {\models} \mathcal{G}_{[\Istart, \Iend]}\,\mtl$; it indicates that $\forall\distance\,{\in}\,[\Istart, \Iend] ~\m{and}~ (\history, \timepoint\plus\distance)\models\mtl$, 
which means that 
$\exists \interval^\prime.~ \timepoint\plus\distance\,{\in}\, \interval^\prime ~\m{and} ~\llbracket \nm(\interval^\prime) \rrbracket_{\Prolog} {=} \m{true}$
\\
Next, from $[\trans\text{-}\m{Globally}]$, 
we obtain \\ 
$\llbracket \nmNEW([\interval^\prime_\m{start}\text{-}\Istart, \interval^\prime_\m{end}\text{-}\Iend]) \rrbracket_{\Prolog} {=} \m{true}$,  and thus \\  $\timepoint\,{\in}\,[\interval^\prime_\m{start}\text{-}\Istart, \interval^\prime_\m{end}\text{-}\Iend]$; 
thus, the rule is complete.

\item  Next:
{
\small 
\begin{align*}
\frac{
\begin{matrix}
\widetilde{\drule} {=} 
[\nmNEW([\interval^\prime_\m{start}\text{-}1, \interval^\prime_\m{end}\text{-}1]) \hornarrow \nm(\interval^\prime).]
\end{matrix}
}{\encoding {\mathcal{N}\,\mtl}{\nmNEW}{\widetilde{\drule} }}\ [\trans\text{-}\m{Next}]
\end{align*}
\vspace{-1mm}
\begin{align*}
\input{sementics_rules/Next_sementic}
\end{align*}
\vspace{-8mm}
}

In $[\trans\text{-}\m{Next}]$  with 
$\mathcal{N}\,\mtl$, \\
$\forall \interval^{\prime\prime}.~\llbracket \nmNEW(\interval^{\prime\prime}) \rrbracket_{\Prolog} {=} \m{true}$, 
its premise indicates that \\
$\llbracket  \nm([\interval^{\prime\prime}_\m{start}\plus 1, \interval^{\prime\prime}_\m{end}\plus 1])\rrbracket_{\history} {=} \m{true}$. \\
Next, from the semantic definition, we have \\
$\forall  \timepoint\,{\in}\,\interval^{\prime\prime}, 
(\history, \timepoint) {\models} \mathcal{N}\,\mtl$; thus the rule is sound. \\
From the semantic definition, $\forall   
(\history, \timepoint) {\models} \mathcal{N}\,\mtl$, \\ 
it indicates that $ (\history, \timepoint\plus 1)\models\mtl$, which means that \\ 
$\exists \interval^\prime.~ \timepoint\plus1\,{\in}\, \interval^\prime ~\m{and} ~\llbracket \nm(\interval^\prime) \rrbracket_{\Prolog} {=} \m{true}$.\\
Next, from $[\trans\text{-}\m{Next}]$, 
we obtain  \\
$\llbracket \nmNEW([\interval^\prime_\m{start}\text{-}1, \interval^\prime_\m{end}\text{-}1]) \rrbracket_{\Prolog} {=} \m{true}$, and thus \\  $\timepoint\,{\in}\,[\interval^\prime_\m{start}\text{-}1, \interval^\prime_\m{end}\text{-}1]$; 
thus, the rule is complete.

\item  Until: 
{
\small 
\begin{align*}
\frac{
\begin{matrix}
\encoding{\mtl_1}{\nm_1}{\widetilde{\drule}_1}
\qquad 
\encoding{\mtl_2}{\nm_2}{\widetilde{\drule}_2}
\\[0.2em]
\widetilde{\drule}_3{=} [\m{helper1}([\interval^\prime_{\m{start}}\plus\interval_{\m{start}}, \interval^\prime_{\m{end}}\plus1]) \hornarrow 
\nm_1(\interval^\prime).]
\\[0.2em]
\widetilde{\drule}_4{=} [\m{helper2}(\interval_1\,{\cap}\,\interval_2) \hornarrow 
\m{helper1}(\interval_1), 
\nm_2(\interval_2).] 
\\[0.2em]
\encoding {\mathcal{F}_\interval\,(\m{helper2})}{\nm_f}{\widetilde{\drule}_5 }
\\[0.2em]
\widetilde{\drule}_6{=} [\nmNEW(\interval_1\cap \interval_2) \hornarrow 
\nm_1(\interval_1), 
\nm_
f(\interval_2). ] 
\end{matrix}
}{\encoding{\mtl_1\,\mathcal{U}_\interval\,\mtl_2}{\nmNEW}{\widetilde{\drule}_1\cup \widetilde{\drule}_2\cup
\widetilde{\drule}_3\cup
\widetilde{\drule}_4\cup
\widetilde{\drule}_5\cup
\widetilde{\drule}_6}}\ [\trans\text{-}\m{Until}]
%\shil{
%~2. ~what's ~the~ definition ~\interval ~in~ \mathcal{F}? }
%\\ \shil{~3. ~what's ~the ~meaning ~of ~;?}\text{\syh{to~construct~list~from~single~rules}}
\end{align*}
%\vspace{-1mm}
\begin{align*}
\input{sementics_rules/Until_sementic}
\end{align*}
\vspace{-8mm}
}

In $[\trans\text{-}\m{Until}]$  with 
$\mtl_1\,\mathcal{U}_{[\Istart, \Iend]}\,\mtl_2$, \\
$\forall \interval^{\prime}.~\llbracket \nmNEW(\interval^{\prime}) \rrbracket_{\Prolog} {=} \m{true}$, 
its premise indicates that \\
$\forall \timepoint\,{\in}\,\interval^{\prime}, 
\m{exists~\distance}.~ \distance\,{\in}\, {[\Istart, \Iend]}  ~ \m{and}~ $\\ 
$
(\history, k)\models \mtl_1 ~\m{forall}~ 
k~\m{with} ~\timepoint{<}k{<}(\timepoint\plus\distance)
~ \m{and}~(\history, \timepoint\plus\distance)\models\mtl_2 $, \\
guaranteed by the helper functions $\m{helper1}$, $\m{helper2}$, and $\nm_f$.  Next, from the semantic definition, we have \\
$(\history, \timepoint) {\models} \mtl_1\,\mathcal{U}_{[\Istart, \Iend]}\,\mtl_2$; thus the rule is sound. \\
From the semantic definition, $\forall   
(\history, \timepoint) {\models} \mtl_1\,\mathcal{U}_{[\Istart, \Iend]}\,\mtl_2$, \\ it indicates that $ \m{exists~\distance}.~ \distance\,{\in}\,{[\Istart, \Iend]}  ~ \m{and}~ (\history, \timepoint\plus\distance)\models\mtl_2 ~ \m{and}~(\history, k)\models \mtl_1 ~\m{forall}~ 
k~\m{with} ~\timepoint{<}k{<}(\timepoint\plus\distance)$. \\ 
Next, from $[\trans\text{-}\m{Until}]$, 
$\m{helper1}$ produces the superset of the possible values of $\timepoint{\plus}\distance$ which satisfy the first constrain, then $\m{helper2}$ produces the exact set of the possible values of $\timepoint{\plus}\distance$ which also satisfy the second constrain. 
Lastly, $\nmNEW$ produces the exact set of the possible values of $\timepoint$; thus, the rule is complete. 

\item $\mtl_1  
\,\mathcal{U}_{[0, 0]} \,  \mtl_2$ $\equiv$ $\mtl_2$: 
{
\small 
\begin{align*}
\input{sementics_rules/Until_sementic}
\end{align*}
\vspace{-8mm}
}

By instantiating the above semantic rule for Until operators with $\interval{=}[0, 0]$, we obtain the following semantic rule: 

{
\small 
\begin{align*}
(\history, \timepoint) &\models \mtl_1 \, \mathcal{U}_{[0, 0]} \,\mtl_2  & \m{iff}&~  \m{exists~\distance}.~ \distance{=}0  ~ \m{and}~ (\history, \timepoint\plus 0)\models\mtl_2 ~ \m{and}
\\[0.1em] 
&&& ~ 
(\history, k)\models \mtl_1 ~\m{forall}~ 
k~\m{with} ~\timepoint{<}k{<}(\timepoint\plus 0)
\end{align*}}

Which is essentially: 

{
\small 
\begin{align*}
(\history, \timepoint) &\models \mtl_1 \, \mathcal{U}_{[0, 0]} \,\mtl_2  & \m{iff}&~   (\history, \timepoint)\models\mtl_2 
\end{align*}}

Thus, the conclusion $\mtl_1  
\,\mathcal{U}_{[0, 0]} \,  \mtl_2$ $\equiv$ $\mtl_2$ is sound and complete. 

\item  Negation:
{
\small 
\begin{align*}
\frac{
\begin{matrix}
\encoding{\mtl}{\nm}{\widetilde{\drule}_1}
\\ 
\widetilde{\drule}{=}[\nmNEW(\interval) \hornarrow
\m{findall}(\interval_1, \nm), \m{compl}(\interval_1, \interval).]
\end{matrix}
}{
\encoding{\neg\mtl}{\nmNEW}{
\widetilde{\drule}_1\,{\cup}\,\widetilde{\drule}}
}\ [\trans\text{-}\m{Neg}]
\end{align*}
\vspace{-1mm}
\begin{align*}
\input{sementics_rules/Neg_semnetic}
\end{align*}
\vspace{-8mm}
}

In $[\trans\text{-}\m{Neg}]$  with 
$\neg\,\mtl$, \\
$\forall \interval.~\llbracket \nmNEW(\interval) \rrbracket_{\Prolog} {=} \m{true}$, 
its premise indicates that \\ 
$\forall \interval_1.~ \nm(\interval_1), \m{and} ~ \interval \cap \interval_1 \,{=}\, \emptyset$. 
\\
Next, from the semantic definition, we have \\
$\forall  \timepoint\,{\in}\,\interval, 
(\history, \timepoint) {\models} \neg\,\mtl$; thus the rule is sound. \\
From the semantic definition, $\forall   
(\history, \timepoint) {\models} \neg\,\mtl$, it indicates that $ (\history, \timepoint){\not\models}\mtl$, 
which means that 
$\forall \interval'. ~ \timepoint\,{\not\in}\,\interval'$ and $\llbracket \nm(\interval^\prime) \rrbracket_{\Prolog} {=} \m{true}$. 
\\
Next, from $[\trans\text{-}\m{Neg}]$, 
we obtain  \\
$\exists\interval.~ \timepoint\,{\in}\,\interval, \interval \cap (\m{findall}(\interval_1, \nm)) {=} \emptyset,$ and $ \llbracket \nmNEW(\interval) \rrbracket_{\Prolog} {=} \m{true}$; 
thus, the rule is complete. 

\item Disjunction:
{
\small 
\begin{align*}
\frac{
\begin{matrix}
[\trans\text{-}\m{Disj}]\\
\encoding{\mtl_1}{\nm_1}{\widetilde{\drule}_1}
\qquad 
\encoding{\mtl_2}{\nm_1}{\widetilde{\drule}_2}
\\
\widetilde{\drule}{=}[\nmNEW(\interval_1\,{\cup}\,\interval_2) \hornarrow
\m{findall}(\interval_1, \nm_1), \m{findall}(\interval_2, \nm_2)]
\end{matrix}
}{
\encoding{\mtl_1{\vee}\mtl_2}{\nmNEW}{ \widetilde{\drule}_1\,{\cup}\,\widetilde{\drule}_2\,{\cup}\,\widetilde{\drule}}
}
\end{align*}
%\vspace{-1mm}
\begin{align*}
\input{sementics_rules/Disj_sementic}
\end{align*}
\vspace{2mm}
}

In $[\trans\text{-}\m{Disj}]$  with 
$\mtl_1{\vee}\mtl_2$, \\
$\forall \interval.~\llbracket \nmNEW(\interval) \rrbracket_{\Prolog} {=} \m{true}$, 
its premise indicates that \\ 
$\forall \interval_1. \forall \interval_2.~ \nm_1(\interval_1), \nm_2(\interval_2)~ \m{and} ~  \interval {=} \interval_1 \cup \interval_2$. 
Next, from the semantic definition, we have \\
$\forall  \timepoint\,{\in}\,\interval, 
(\history, \timepoint) {\models} \mtl_1 \vee \mtl_2$; thus the rule is sound. \\
From the semantic definition, $\forall   
(\history, \timepoint) {\models} \mtl_1 \vee \mtl_2$, it indicates that $(\history, \timepoint)\models\mtl_1$ or $(\history, \timepoint)\models\mtl_2$.\\
Next, from $[\trans\text{-}\m{Disj}]$, 
$\exists \interval.~\llbracket \nm_1(\interval) \rrbracket_{\Prolog} {=} \m{true}$ or $\llbracket \nm_2(\interval) \rrbracket_{\Prolog} {=} \m{true}$
we obtain  \\
$\llbracket \nmNEW(\interval) \rrbracket_{\Prolog} {=} \m{true}$,  and $\timepoint\,{\in}\,\interval$; 
thus, the rule is complete. 

\item Conjunction:
{
\small 
\begin{align*}
\frac{
\begin{matrix}
[\trans\text{-}\m{Conj}]\\
\encoding{\mtl_1}{\nm_1}{\widetilde{\drule}_1}
\qquad 
\encoding{\mtl_2}{\nm_1}{\widetilde{\drule}_2}
\\
\widetilde{\drule}{=}[\nmNEW(\interval_1\,{\cap}\,\interval_2) \hornarrow
\m{findall}(\interval_1, \nm_1), \m{findall}(\interval_2, \nm_2)]
\end{matrix}
}{
\encoding{\mtl_1{\wedge}\mtl_2}{\nmNEW}{ \widetilde{\drule}_1\,{\cup}\,\widetilde{\drule}_2\,{\cup}\,\widetilde{\drule}}
}
\end{align*}
%\vspace{-1mm}
\begin{align*}
\input{sementics_rules/Conj_sementic}
\end{align*}
\vspace{-2mm}
}

In $[\trans\text{-}\m{Conj}]$  with 
$\mtl_1{\wedge}\mtl_2$, \\
$\forall \interval.~\llbracket \nmNEW(\interval) \rrbracket_{\Prolog} {=} \m{true}$, 
its premise indicates that \\ 
$\forall \interval_1. \forall \interval_2.~ \nm_1(\interval_1), \nm_2(\interval_2)~ \m{and} ~  \interval {=} \interval_1 \cap \interval_2$. 
Next, from the semantic definition, we have \\
$\forall  \timepoint\,{\in}\,\interval, 
(\history, \timepoint) {\models} \mtl_1 \wedge \mtl_2$; thus the rule is sound. \\
From the semantic definition, $\forall   
(\history, \timepoint) {\models} \mtl_1 \wedge \mtl_2$, it indicates that $(\history, \timepoint)\models\mtl_1$ and $(\history, \timepoint)\models\mtl_2$.\\
Next, from $[\trans\text{-}\m{Conj}]$, 
$\exists \interval.~\llbracket \nm_1(\interval) \rrbracket_{\Prolog} {=} \m{true}$ and $\llbracket \nm_2(\interval) \rrbracket_{\Prolog} {=} \m{true}$
we obtain  \\
$\llbracket \nmNEW(\interval) \rrbracket_{\Prolog} {=} \m{true}$,  and $\timepoint\,{\in}\,\interval$; 
thus, the rule is complete. 
\end{enumerate}
\vspace{3mm}

All the encoding rules are sound and complete. 

\end{proof}
